# Supplementary material for: VaLID: Variable-Length Input Diffusion for Novel View Synthesis
Source: arXiv:2312.08892 source file (2023-12-14)
Supplement: Supplementary file 1 [file supp_temporal_consistency_1.tex]

\begin{figure*}[t!]
\centering
\subfloat[GT]{
\begin{minipage}[t]{0.125\linewidth}
\centering
\includegraphics[width=\linewidth]
{{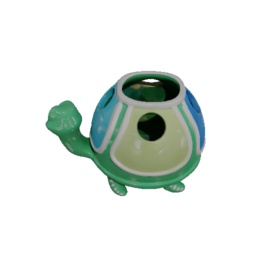}}\\
\includegraphics[width=\linewidth]
{{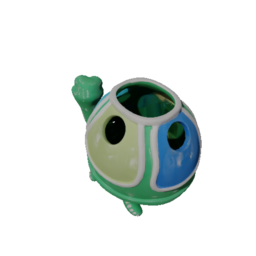}}\\
\includegraphics[width=\linewidth]
{{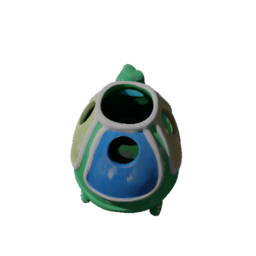}}\\
\includegraphics[width=\linewidth]
{{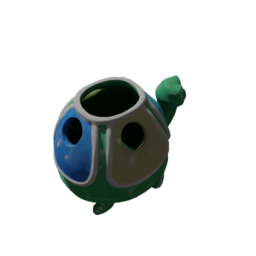}}\\
\includegraphics[width=\linewidth]
{{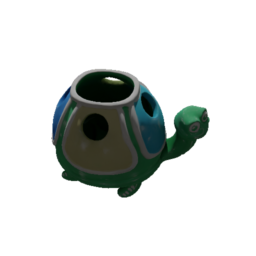}}\\
\includegraphics[width=\linewidth]
{{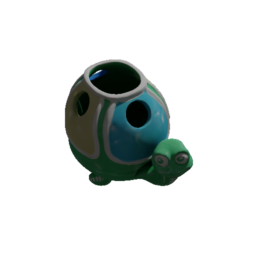}}\\
\includegraphics[width=\linewidth]
{{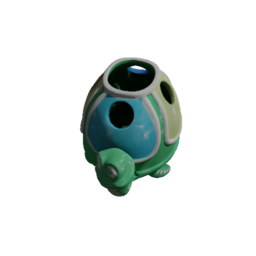}}\\
\includegraphics[width=\linewidth]
{{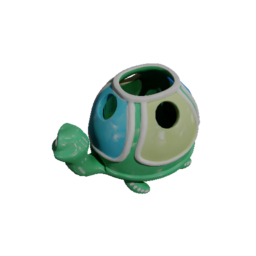}}\\
\includegraphics[width=\linewidth]
{{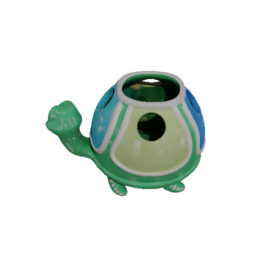}}\\
\end{minipage}
}
\hspace{-5mm}
\subfloat[Zero123]{
\begin{minipage}[t]{0.125\linewidth}
\centering
\includegraphics[width=\linewidth]
{{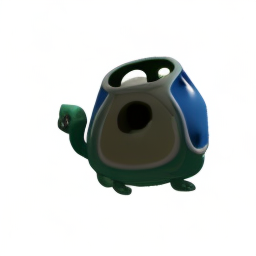}}\\
\includegraphics[width=\linewidth]
{{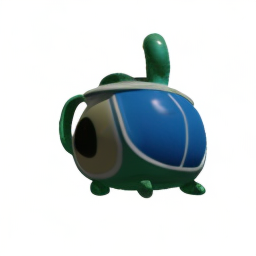}}\\
\includegraphics[width=\linewidth]
{{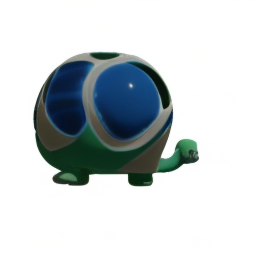}}\\
\includegraphics[width=\linewidth]
{{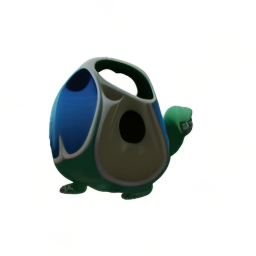}}\\
\includegraphics[width=\linewidth]
{{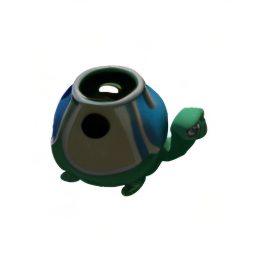}}\\
\includegraphics[width=\linewidth]
{{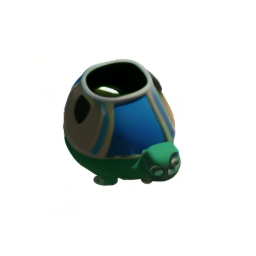}}\\
\includegraphics[width=\linewidth]
{{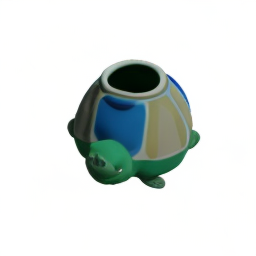}}\\
\includegraphics[width=\linewidth]
{{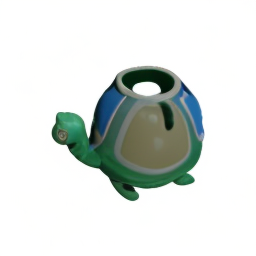}}\\
\includegraphics[width=\linewidth]
{{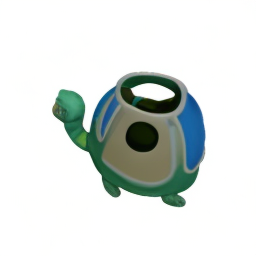}}\\
\end{minipage}
}
\hspace{-5mm}
\subfloat[VaLID 1v]{
\begin{minipage}[t]{0.125\linewidth}
\centering
\includegraphics[width=\linewidth]
{{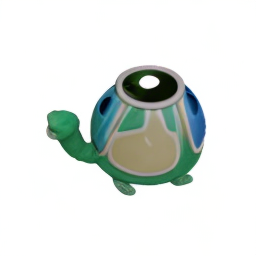}}\\
\includegraphics[width=\linewidth]
{{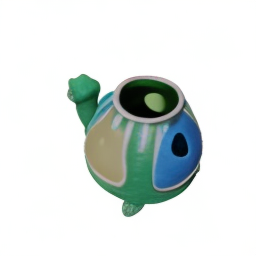}}\\
\includegraphics[width=\linewidth]
{{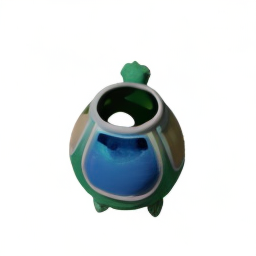}}\\
\includegraphics[width=\linewidth]
{{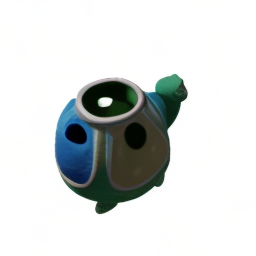}}\\
\includegraphics[width=\linewidth]
{{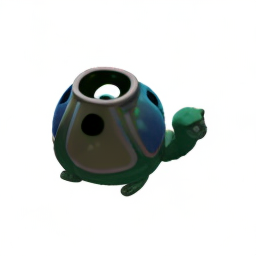}}\\
\includegraphics[width=\linewidth]
{{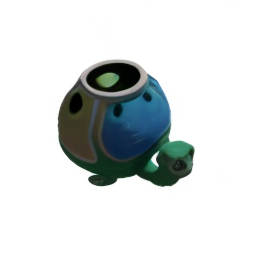}}\\
\includegraphics[width=\linewidth]
{{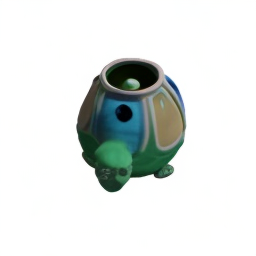}}\\
\includegraphics[width=\linewidth]
{{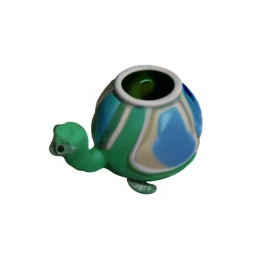}}\\
\includegraphics[width=\linewidth]
{{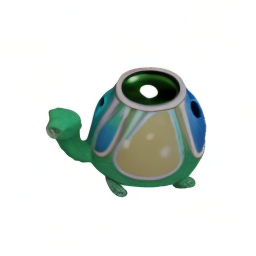}}\\
\end{minipage}
}
\hspace{-5mm}
\subfloat[VaLID 4v]{
\begin{minipage}[t]{0.125\linewidth}
\centering
\includegraphics[width=\linewidth]
{{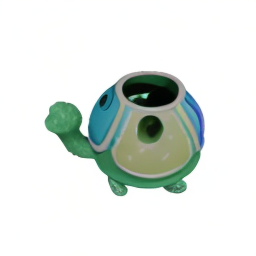}}\\
\includegraphics[width=\linewidth]
{{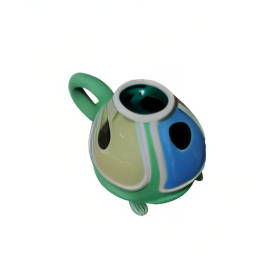}}\\
\includegraphics[width=\linewidth]
{{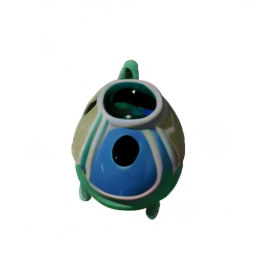}}\\
\includegraphics[width=\linewidth]
{{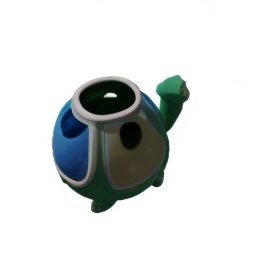}}\\
\includegraphics[width=\linewidth]
{{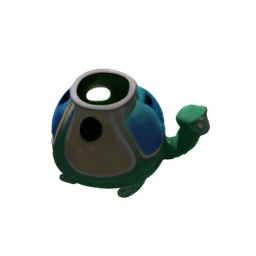}}\\
\includegraphics[width=\linewidth]
{{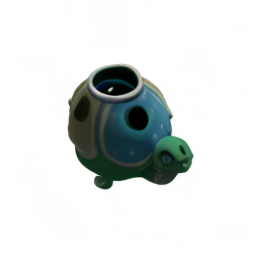}}\\
\includegraphics[width=\linewidth]
{{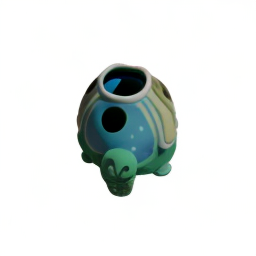}}\\
\includegraphics[width=\linewidth]
{{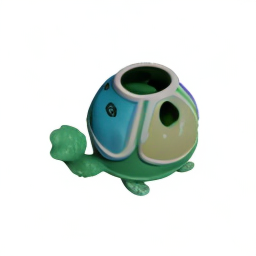}}\\
\includegraphics[width=\linewidth]
{{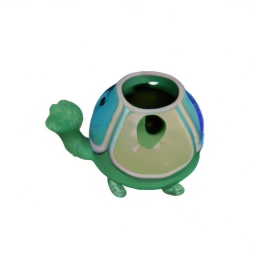}}\\
\end{minipage}
}
\subfloat[GT]{
\begin{minipage}[t]{0.125\linewidth}
\centering
\includegraphics[width=\linewidth]
{{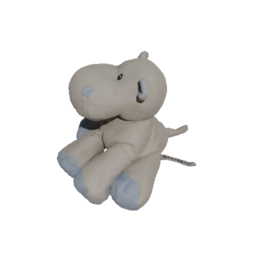}}\\
\includegraphics[width=\linewidth]
{{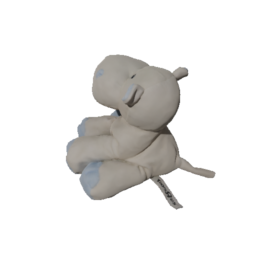}}\\
\includegraphics[width=\linewidth]
{{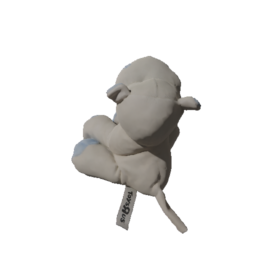}}\\
\includegraphics[width=\linewidth]
{{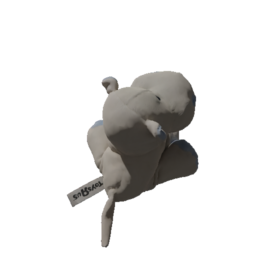}}\\
\includegraphics[width=\linewidth]
{{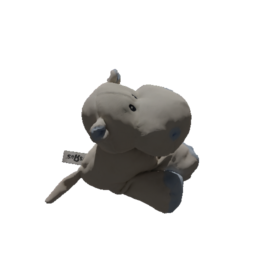}}\\
\includegraphics[width=\linewidth]
{{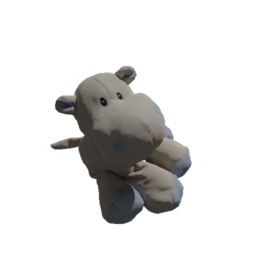}}\\
\includegraphics[width=\linewidth]
{{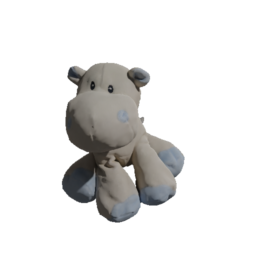}}\\
\includegraphics[width=\linewidth]
{{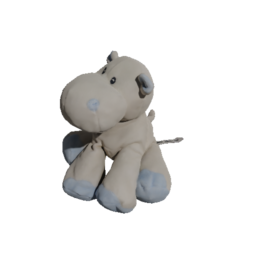}}\\
\includegraphics[width=\linewidth]
{{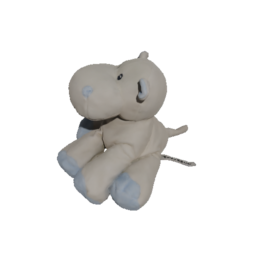}}\\
\end{minipage}
}
\hspace{-5mm}
\subfloat[Zero123]{
\begin{minipage}[t]{0.125\linewidth}
\centering
\includegraphics[width=\linewidth]
{{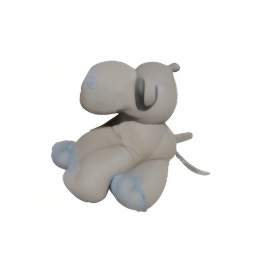}}\\
\includegraphics[width=\linewidth]
{{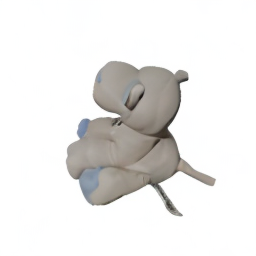}}\\
\includegraphics[width=\linewidth]
{{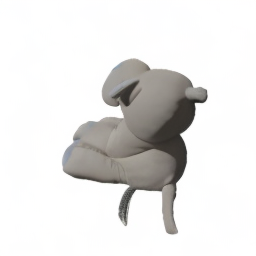}}\\
\includegraphics[width=\linewidth]
{{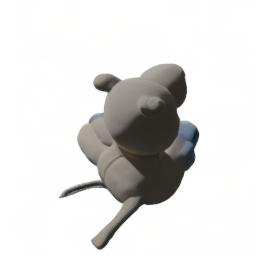}}\\
\includegraphics[width=\linewidth]
{{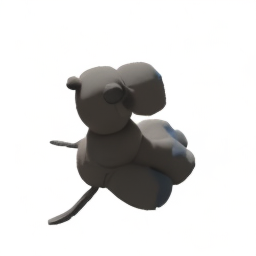}}\\
\includegraphics[width=\linewidth]
{{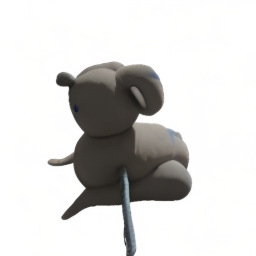}}\\
\includegraphics[width=\linewidth]
{{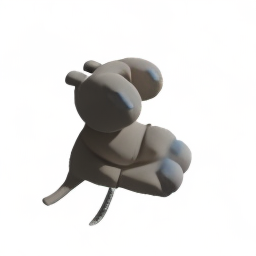}}\\
\includegraphics[width=\linewidth]
{{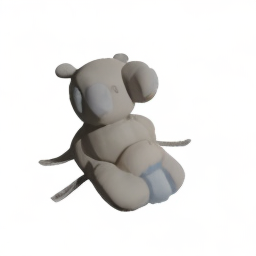}}\\
\includegraphics[width=\linewidth]
{{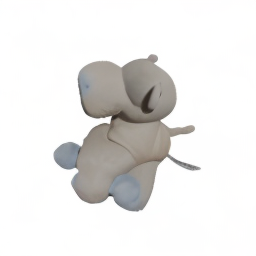}}\\
\end{minipage}
}
\hspace{-5mm}
\subfloat[VaLID 1v]{
\begin{minipage}[t]{0.125\linewidth}
\centering
\includegraphics[width=\linewidth]
{{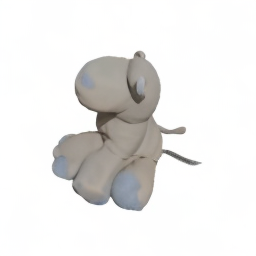}}\\
\includegraphics[width=\linewidth]
{{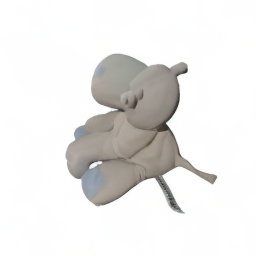}}\\
\includegraphics[width=\linewidth]
{{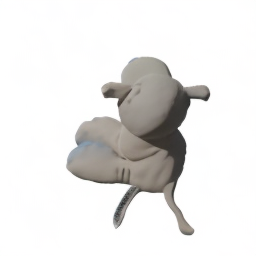}}\\
\includegraphics[width=\linewidth]
{{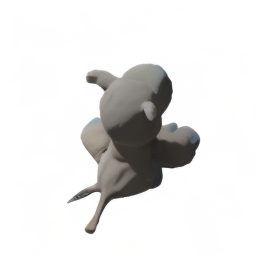}}\\
\includegraphics[width=\linewidth]
{{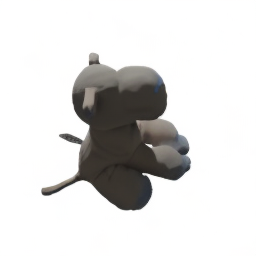}}\\
\includegraphics[width=\linewidth]
{{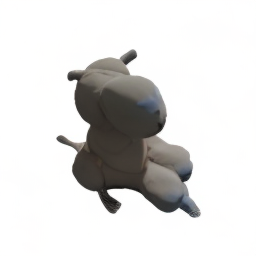}}\\
\includegraphics[width=\linewidth]
{{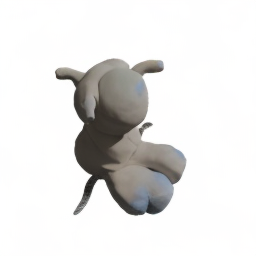}}\\
\includegraphics[width=\linewidth]
{{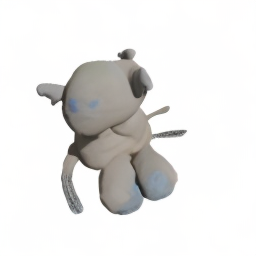}}\\
\includegraphics[width=\linewidth]
{{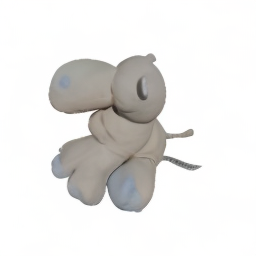}}\\
\end{minipage}
}
\hspace{-5mm}
\subfloat[VaLID 4v]{
\begin{minipage}[t]{0.125\linewidth}
\centering
\includegraphics[width=\linewidth]
{{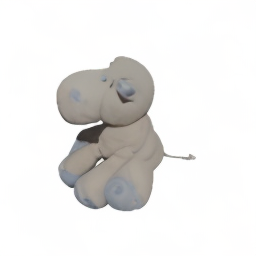}}\\
\includegraphics[width=\linewidth]
{{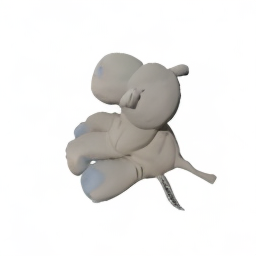}}\\
\includegraphics[width=\linewidth]
{{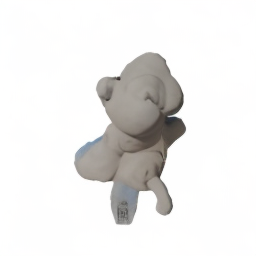}}\\
\includegraphics[width=\linewidth]
{{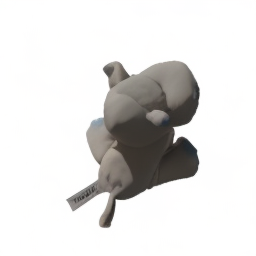}}\\
\includegraphics[width=\linewidth]
{{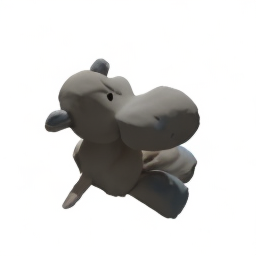}}\\
\includegraphics[width=\linewidth]
{{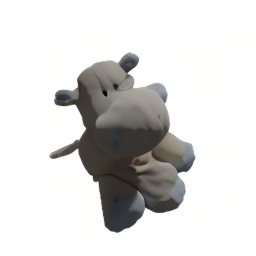}}\\
\includegraphics[width=\linewidth]
{{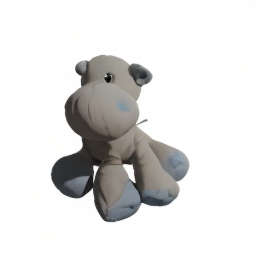}}\\
\includegraphics[width=\linewidth]
{{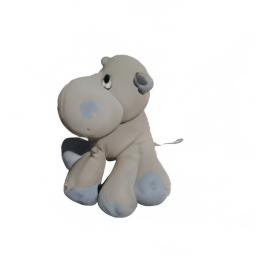}}\\
\includegraphics[width=\linewidth]
{{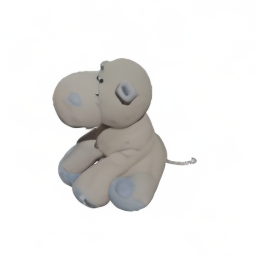}}\\
\end{minipage}
}
% \vspace{-3mm}
\caption{
Temporal consistency in the rendered video. The frames are in order from top to bottom.
}
\label{fig:temporal_consistency}
\vspace{-5mm}
\end{figure*}
