# Supplementary material for: VaLID: Variable-Length Input Diffusion for Novel View Synthesis
Source: arXiv:2312.08892 source file (2023-12-14)
Supplement: Supplementary file 3 [file supp_qvis_2.tex]

\begin{figure*}[t!]
\centering
\hspace{-5mm}
\subfloat[Target View]{
\begin{minipage}[t]{0.16\linewidth}
\centering
\includegraphics[width=\linewidth]{{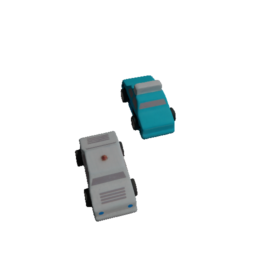}}\\
\vspace{-3mm}
\includegraphics[width=\linewidth]{{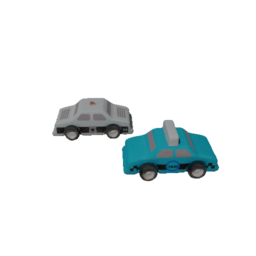}}\\
\vspace{-3mm}
% \includegraphics[width=\linewidth]{{imgs/supp/zero123_vs_valid/target/CITY_TAXI_POLICE_CAR_012.png}}\\
% \vspace{-3mm}
% \includegraphics[width=\linewidth]{{imgs/supp/zero123_vs_valid/target/CITY_TAXI_POLICE_CAR_015.png}}\\
\vspace{-3mm}
\includegraphics[width=\linewidth]{{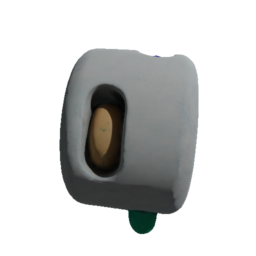}}\\
\vspace{-3mm}
\includegraphics[width=\linewidth]{{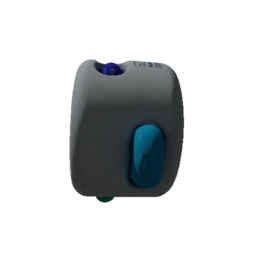}}\\
\vspace{-3mm}
\includegraphics[width=\linewidth]{{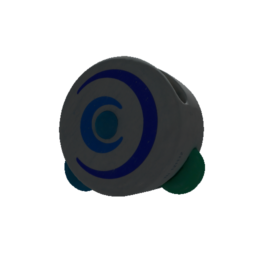}}\\
\vspace{-3mm}
\includegraphics[width=\linewidth]{{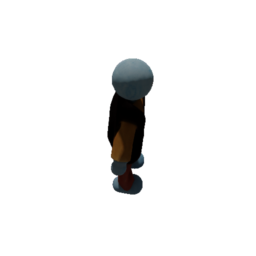}}\\
\vspace{-3mm}
\includegraphics[width=\linewidth]{{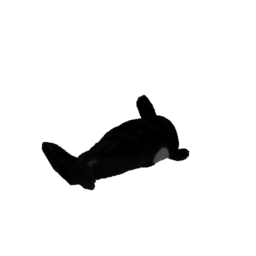}}\\
\vspace{-3mm}
\includegraphics[width=\linewidth]{{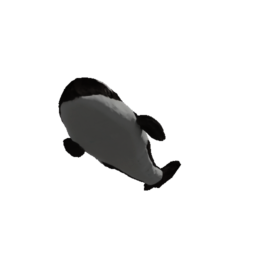}}\\
\vspace{-3mm}
\end{minipage}
}
\hspace{-5mm}
\subfloat[Zero123\cite{liu2023zero}]{
\begin{minipage}[t]{0.16\linewidth}
\centering
\includegraphics[width=\linewidth]{{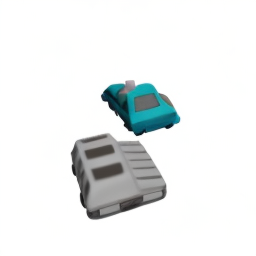}}\\
\vspace{-3mm}
\includegraphics[width=\linewidth]{{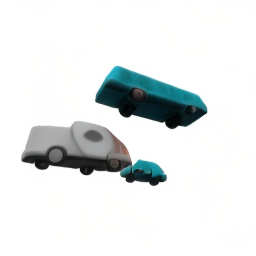}}\\
\vspace{-3mm}
% \includegraphics[width=\linewidth]{{imgs/supp/zero123_vs_valid/zero123/CITY_TAXI_POLICE_CAR_012.png}}\\
% \vspace{-3mm}
% \includegraphics[width=\linewidth]{{imgs/supp/zero123_vs_valid/zero123/CITY_TAXI_POLICE_CAR_015.png}}\\
\vspace{-3mm}
\includegraphics[width=\linewidth]{{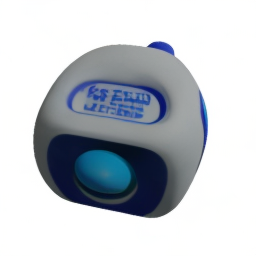}}\\
\vspace{-3mm}
\includegraphics[width=\linewidth]{{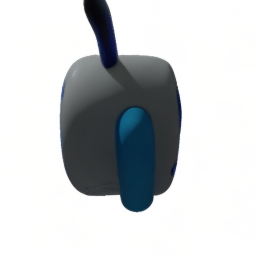}}\\
\vspace{-3mm}
\includegraphics[width=\linewidth]{{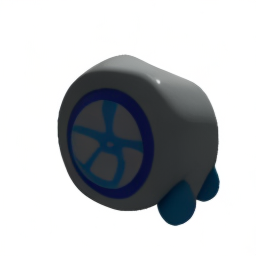}}\\
\includegraphics[width=\linewidth]{{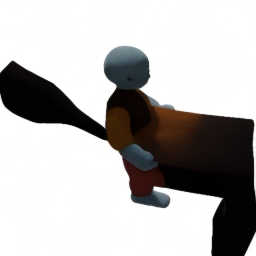}}\\
\vspace{-3mm}
\includegraphics[width=\linewidth]{{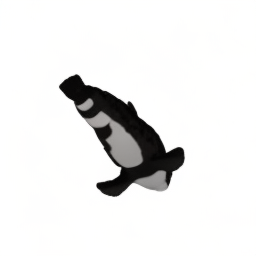}}\\
\vspace{-3mm}
\includegraphics[width=\linewidth]{{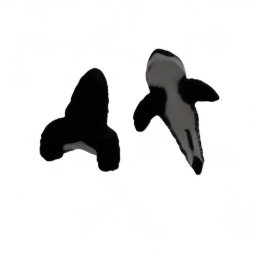}}\\
\vspace{-3mm}
\end{minipage}
}
\hspace{-5mm}
\subfloat[VaLID (1 view)]{
\begin{minipage}[t]{0.16\linewidth}
\centering
\includegraphics[width=\linewidth]{{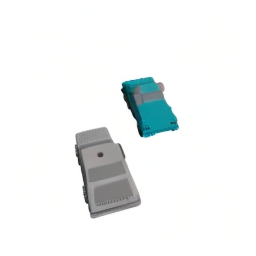}}\\
\vspace{-3mm}
\includegraphics[width=\linewidth]{{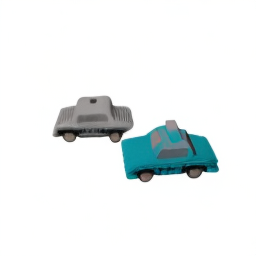}}\\
\vspace{-3mm}
% \includegraphics[width=\linewidth]{{imgs/supp/zero123_vs_valid/valid_v1/CITY_TAXI_POLICE_CAR_012.png}}\\
% \vspace{-3mm}
% \includegraphics[width=\linewidth]{{imgs/supp/zero123_vs_valid/valid_v1/CITY_TAXI_POLICE_CAR_015.png}}\\
\vspace{-3mm}
\includegraphics[width=\linewidth]{{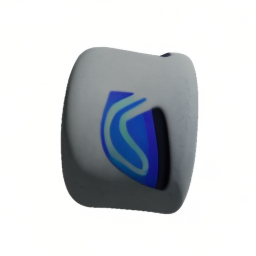}}\\
\vspace{-3mm}
\includegraphics[width=\linewidth]{{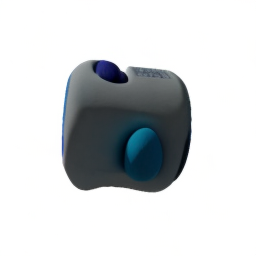}}\\
\vspace{-3mm}
\includegraphics[width=\linewidth]{{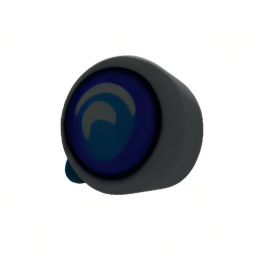}}\\
\includegraphics[width=\linewidth]{{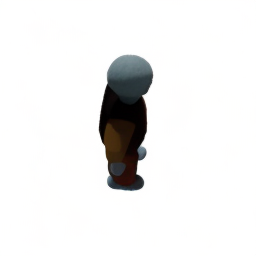}}\\
\vspace{-3mm}
\includegraphics[width=\linewidth]{{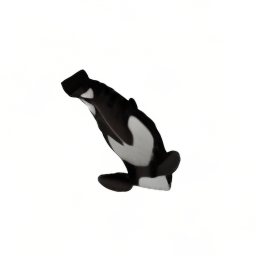}}\\
\vspace{-3mm}
\includegraphics[width=\linewidth]{{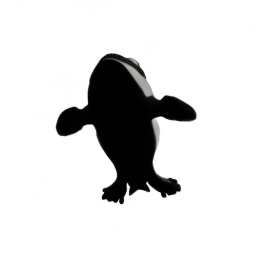}}\\
\vspace{-3mm}
\end{minipage}
}
\hspace{-5mm}
\subfloat[VaLID (2 view)]{
\begin{minipage}[t]{0.16\linewidth}
\centering
\includegraphics[width=\linewidth]{{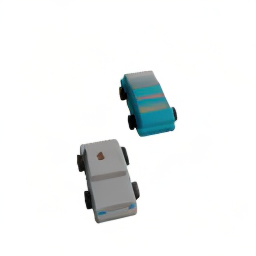}}\\
\vspace{-3mm}
\includegraphics[width=\linewidth]{{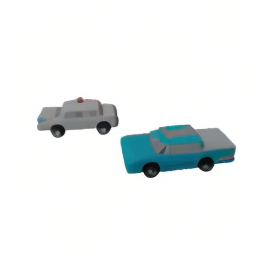}}\\
\vspace{-3mm}
% \includegraphics[width=\linewidth]{{imgs/supp/zero123_vs_valid/valid_v2/CITY_TAXI_POLICE_CAR_012.png}}\\
% \vspace{-3mm}
% \includegraphics[width=\linewidth]{{imgs/supp/zero123_vs_valid/valid_v2/CITY_TAXI_POLICE_CAR_015.png}}\\
\vspace{-3mm}
\includegraphics[width=\linewidth]{{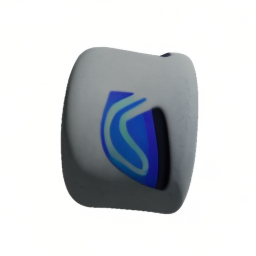}}\\
\vspace{-3mm}
\includegraphics[width=\linewidth]{{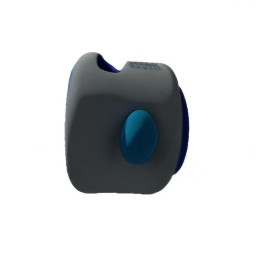}}\\
\vspace{-3mm}
\includegraphics[width=\linewidth]{{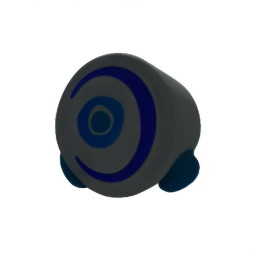}}\\
\includegraphics[width=\linewidth]{{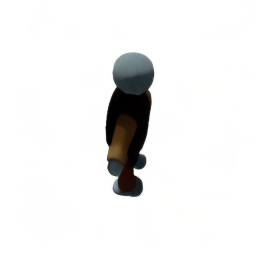}}\\
\vspace{-3mm}
\includegraphics[width=\linewidth]{{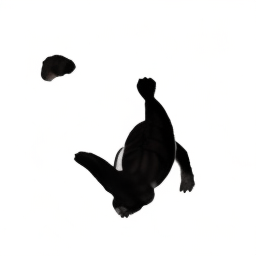}}\\
\vspace{-3mm}
\includegraphics[width=\linewidth]{{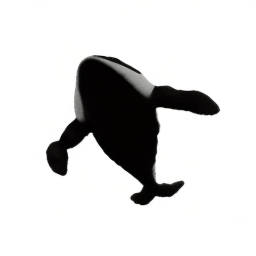}}\\
\vspace{-3mm}
\end{minipage}
}
\hspace{-5mm}
\subfloat[VaLID (3 view)]{
\begin{minipage}[t]{0.16\linewidth}
\centering
\includegraphics[width=\linewidth]{{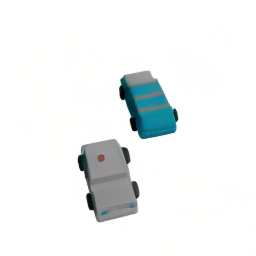}}\\
\vspace{-3mm}
\includegraphics[width=\linewidth]{{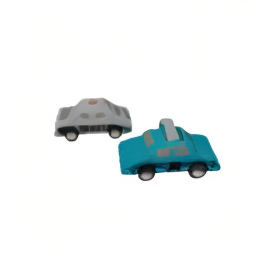}}\\
\vspace{-3mm}
% \includegraphics[width=\linewidth]{{imgs/supp/zero123_vs_valid/valid_v3/CITY_TAXI_POLICE_CAR_012.png}}\\
% \vspace{-3mm}
% \includegraphics[width=\linewidth]{{imgs/supp/zero123_vs_valid/valid_v3/CITY_TAXI_POLICE_CAR_015.png}}\\
\vspace{-3mm}
\includegraphics[width=\linewidth]{{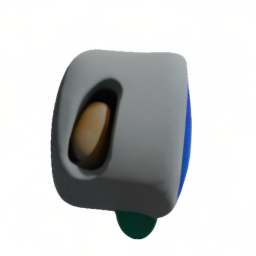}}\\
\vspace{-3mm}
\includegraphics[width=\linewidth]{{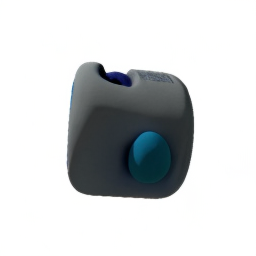}}\\
\vspace{-3mm}
\includegraphics[width=\linewidth]{{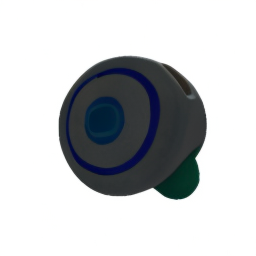}}\\
\includegraphics[width=\linewidth]{{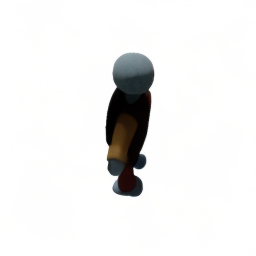}}\\
\vspace{-3mm}
\includegraphics[width=\linewidth]{{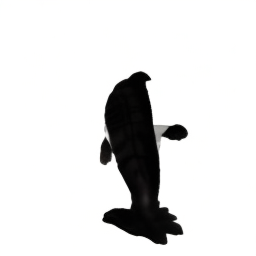}}\\
\vspace{-3mm}
\includegraphics[width=\linewidth]{{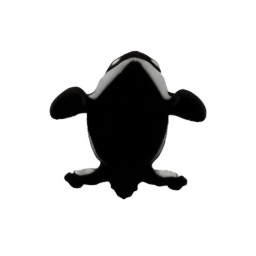}}\\
\vspace{-3mm}
\end{minipage}
}
\hspace{-5mm}
\subfloat[VaLID (4 view)]{
\begin{minipage}[t]{0.16\linewidth}
\centering
\includegraphics[width=\linewidth]{{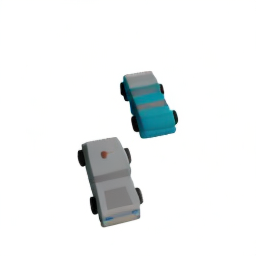}}\\
\vspace{-3mm}
\includegraphics[width=\linewidth]{{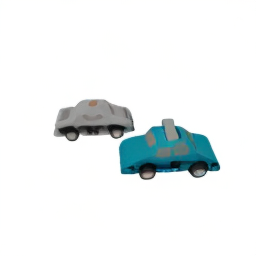}}\\
\vspace{-3mm}
% \includegraphics[width=\linewidth]{{imgs/supp/zero123_vs_valid/valid_v4/CITY_TAXI_POLICE_CAR_012.png}}\\
% \vspace{-3mm}
% \includegraphics[width=\linewidth]{{imgs/supp/zero123_vs_valid/valid_v4/CITY_TAXI_POLICE_CAR_015.png}}\\
\vspace{-3mm}
\includegraphics[width=\linewidth]{{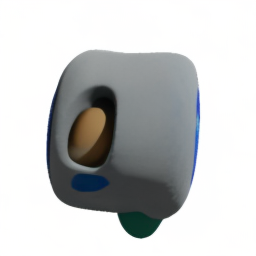}}\\
\vspace{-3mm}
\includegraphics[width=\linewidth]{{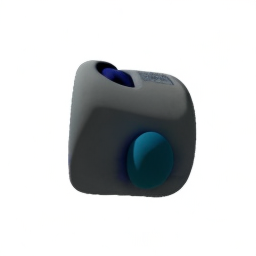}}\\
\vspace{-3mm}
\includegraphics[width=\linewidth]{{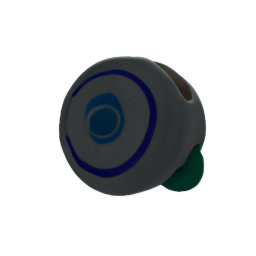}}\\
\includegraphics[width=\linewidth]{{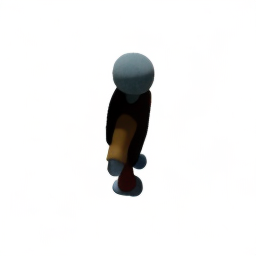}}\\
\vspace{-3mm}
\includegraphics[width=\linewidth]{{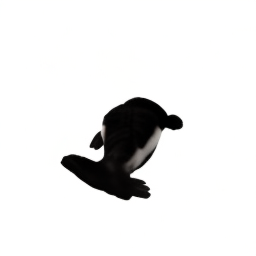}}\\
\vspace{-3mm}
\includegraphics[width=\linewidth]{{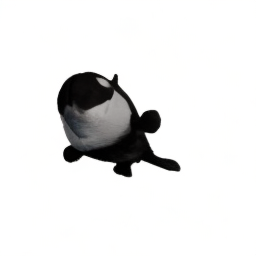}}\\
\vspace{-3mm}
\end{minipage}
}
% \vspace{-3mm}
\caption{
More qualitative results.
}
\label{fig:qvis_2}
\vspace{-5mm}
\end{figure*}
